# Supplementary material for: General quantum-mechanical solution for twisted electrons in a uniform magnetic field
Source: arXiv:2005.06408 source file (2020-12-10)
Supplement: Supplementary file 1 [file SupplementalElectronMagnetic2.pdf]

# Supplemental Material to "General quantum-mechanical solution for twisted electrons in a uniform magnetic field"

Liping Zou, Pengming Zhang, and Alexander J. Silenko

## I. PARAXIAL LAGUERRE-GAUSS BEAMS IN OPTICS

In this Supplemental Material, we expound an introduction of paraxial Laguerre-Gauss (LG) beams in optics. Such beams are now widely used not only in optics but also in electron physics [1–3]. The wave function of the LG beam obtained in optics in the paraxial approximation, $p_\perp << |p_z|$, perfectly agrees with that derived in the framework of quantum mechanics of the Dirac electron (see Ref. [4]). In this approximation, it is convenient to use the Helmholtz equation taking the form

$$(\nabla_\perp^2 + 2ik\partial_z)\boldsymbol{E}(\boldsymbol{r}) = 0, \qquad \nabla_\perp^2 = \nabla^2 - \frac{\partial^2}{\partial z^2}, \tag{S1}$$

where $\boldsymbol{E}(\boldsymbol{r})$ is the electric field strength of an electromagnetic field and $\nabla_\perp^2$ is the transversal part of the Laplace operator $\nabla^2$. In optics, the initial Helmholtz equation is often used in the form

$$(\nabla_\perp^2 - 2ik\partial_z)\boldsymbol{E}(\boldsymbol{r}) = 0. \tag{S2}$$

In this case, some terms in subsequently obtained equations have also different signs. Paraxial Gaussian beams are considered in detail, e.g., in Refs. [5–8]. Derivations are traditionally made for paraxial Hermite-Gauss (HG) beams while LG beams are also discussed. However, it is not a problem to analyze LG beams from the beginning.

For light beams in the free space, one can use the scalar wave function $\Psi$. In the cylindrical coordinates, Eq. (S1) reads

$$\left(\frac{\partial^2}{\partial r^2} + \frac{1}{r}\frac{\partial}{\partial r} + \frac{1}{r^2}\frac{\partial^2}{\partial\phi^2} + 2ik\frac{\partial}{\partial z}\right)\Psi(r,\phi,z) = 0. \tag{S3}$$

For states with a definite OAM, $\Psi(r,\phi,z) = U(r,z)\exp(i\ell\phi)$ and

$$\left(\frac{\partial^2}{\partial r^2} + \frac{1}{r}\frac{\partial}{\partial r} - \frac{\ell^2}{r^2} + 2ik\frac{\partial}{\partial z}\right)U(r,z)\exp(i\ell\phi) = 0. \tag{S4}$$

It is instructive to consider the particular case of the fundamental Gaussian mode first. In this case, $\ell = 0$ and Eq. (S4) reduces to

$$\left(\frac{\partial^2}{\partial r^2} + \frac{1}{r}\frac{\partial}{\partial r} + 2ik\frac{\partial}{\partial z}\right)U(r,z) = 0. \tag{S5}$$

A trial solution of Eq. (S5) can be presented in the form [5, 6]

$$U(r,z) = \exp\left\{i\left[\mathcal{P}(z) + \frac{kr^2}{2q(z)}\right]\right\}. \tag{S6}$$

This solution describes a paraxial spherical wave diverging from a source point located at the origin and observed at the observation point $(r,\phi,z)$. The parameter $\mathcal{P}(z)$ represents a *complex* phase shift which is associated with the propagation of the light beam, and $q(z)$ is a *complex* beam parameter which describes the radius of curvature of the phase front which is spherical near the axis, as well as the Gaussian variation in beam intensity with the distance $r$ from the optic axis [6, 7]. It is convenient to express $q(z)$ in terms of main parameters of the beam [5–8]

$$\frac{1}{q(z)} = \frac{1}{R(z)} + i\frac{2}{kw^2(z)}, \tag{S7}$$

where $R(z)$ is the radius of curvature of the beam wavefront and $w(z)$ is the beam radius. In the simplest case of the fundamental Gaussian mode, the parameter $\mathcal{P}(z)$ can be defined by

$$\exp[i\mathcal{P}(z)] = \frac{1}{w(z)}\exp[-i\Phi_G(z)], \tag{S8}$$

where $\Phi_G(z)$ is the Gouy phase. Thus, the paraxial wave function of a free Gaussian light beam takes the form

$$U(r,z)=\frac{C_G}{w(z)}\exp\left[-\frac{r^2}{w^2(z)}\right]\exp\left\{i\left[\frac{kr^2}{2R(z)}-\Phi_G(z)\right]\right\},\qquad \int U^\dagger(r,z)U(r,z)rdrd\phi=1. \tag{S9}$$

The substitution of this wave function into Eq. (S5) leads to the following relations:

$$\begin{aligned}\nabla_\perp^2\mathbb{A}=\frac{4}{w^2(z)}\left[\frac{r^2}{w^2(z)}-1\right]\mathbb{A},\qquad \nabla_\perp^2U(r,z)=\left\{\frac{4}{w^2(z)}\left[\frac{r^2}{w^2(z)}-1\right]-\frac{k^2r^2}{R^2(z)}+\frac{2ik}{R(z)}\left[1-\frac{2r^2}{w^2(z)}\right]\right\}U(r,z),\\ 2ik\frac{\partial U(r,z)}{\partial z}=\left\{-2ik\frac{w'(z)}{w(z)}\left[1-\frac{2r^2}{w^2(z)}\right]-k^2r^2\left[\frac{1}{R(z)}\right]'+2k\Phi_G'(z)\right\}U(r,z),\qquad \mathbb{A}=\frac{C_G}{w(z)}\exp\left[-\frac{r^2}{w^2(z)}\right].\end{aligned} \tag{S10}$$

As a result, Eq. (S5) takes the form

$$\left\{-\frac{4}{w^2(z)}+r^2\left(\frac{4}{w^4(z)}-k^2\left[\frac{1}{R(z)}\right]'-k^2\frac{1}{R^2(z)}\right)+2ik\left[\frac{1}{R(z)}-\frac{w'(z)}{w(z)}\right]\left[1-\frac{2r^2}{w^2(z)}\right]+2k\Phi_G'(z)\right\}U(r,z)=0. \tag{S11}$$

This equation shows that the following differential equations should be satisfied:

$$\frac{1}{R(z)}=\frac{w'(z)}{w(z)},\qquad \frac{k^2}{R^2(z)}+k^2\left[\frac{1}{R(z)}\right]'=\frac{4}{w^4(z)},\qquad 2k\Phi_G'(z)=\frac{4}{w^2(z)}. \tag{S12}$$

After taking into account the initial conditions $w(0)=w_0$, $w'(0)=0$, one obtains the following expressions for the beam parameters (see Refs. [5–8]):

$$w(z)=w_0\sqrt{1+\frac{z^2}{z_R^2}},\qquad R(z)=z+\frac{z_R^2}{z},\qquad z_R=\frac{kw_0^2}{2},\qquad \Phi_G(z)=\arctan\left(\frac{z}{z_R}\right), \tag{S13}$$

where $z_R$ is the Rayleigh length (Rayleigh range) [5, 7, 8] being the distance along the propagation direction of the beam from the waist to the place where the area of the cross section is doubled. As a result, the wave function of a free Gaussian light beam is defined by Eqs. (S9) and (S13). The normalization constant is equal to

$$C_G=\sqrt{\frac{2}{\pi}}. \tag{S14}$$

The complex radius of curvature of the phase front is equal to

$$q(z)=z-iz_R. \tag{S15}$$

This equation characterizes a paraxial spherical wave.

In the general case, an analysis of Eq. (S3) shows that the wave function is proportional to $r^{|\ell|}$ at $r\to 0$ (cf. Ref. [9]). In this case, a trial solution of Eq. (S4) can be chosen as follows:

$$\begin{aligned}\Psi=\mathbb{A}\exp(i\Phi),\qquad \int\Psi^\dagger\Psi rdrd\phi=1,\qquad \mathbb{A}=\frac{C_{n\ell}}{w(z)}\zeta^{|\ell|/2}F(\zeta)\exp\left(-\frac{\zeta}{2}\right),\qquad \zeta=\frac{2r^2}{w^2(z)},\\ \Phi=l\phi+\frac{kr^2}{2R(z)}-\Phi_G(z),\end{aligned} \tag{S16}$$

where $w(z)$, $F(\zeta)$, $R(z)$, and $\Phi_G(z)$ are not yet specified.

The substitution of the wave function (S16) into Eq. (S5) leads to the following relations:

$$\begin{aligned}\nabla_\perp^2\mathbb{A}\exp(i\ell\phi)=\frac{4}{w^2(z)}\left[\left(\frac{\zeta}{2}-|\ell|-1\right)F(\zeta)+2(|\ell|+1-\zeta)F'(\zeta)+2\zeta F''(\zeta)\right]\frac{\mathbb{A}}{F(\zeta)}\exp(i\ell\phi),\\ \nabla_\perp^2\Psi=\frac{4}{w^2(z)}\left[\left(\frac{\zeta}{2}-|\ell|-1\right)F(\zeta)+2(|\ell|+1-\zeta)F'(\zeta)+2\zeta F''(\zeta)\right]\frac{\Psi}{F(\zeta)}\\ +\left[\frac{2ik(|\ell|+1)}{R(z)}F(\zeta)+\frac{4ikr^2}{w^2(z)R(z)}\Big(2F'(\zeta)-F(\zeta)\Big)-\frac{k^2r^2}{R^2(z)}F(\zeta)\right]\frac{\Psi}{F(\zeta)},\\ 2ik\frac{\partial\Psi}{\partial z}=\left\{-4ikr^2\frac{w'(z)}{w^3(z)}\Big(2F'(\zeta)-F(\zeta)\Big)+\left(-2ik\Big(|\ell|+1\Big)\frac{w'(z)}{w(z)}-k^2r^2\left[\frac{1}{R(z)}\right]'+2k\Phi_G'(z)\right)F(\zeta)\right\}\frac{\Psi}{F(\zeta)},\end{aligned} \tag{S17}$$

where $F'(\zeta) \equiv dF(\zeta)/(d\zeta)$. As a result, Eq. (S4) takes the form

$$\left\{ \frac{8}{w^2(z)}\Big[\zeta F''(\zeta) + \big(|\ell|+1-\zeta\big)F'(\zeta)\Big] + \frac{4}{w^2(z)}\left(\frac{\zeta}{2} - |\ell| - 1\right)F(\zeta) + \left(2k\Phi'_G(z) - \frac{k^2r^2}{R^2(z)} - k^2r^2\left[\frac{1}{R(z)}\right]'\right)F(\zeta) \right.$$
$$\left. +2ik\left[\frac{1}{R(z)} - \frac{w'(z)}{w(z)}\right]\left[\big(|\ell|+1\big)F(\zeta) + \frac{2r^2}{w^2(z)}\Big(2F'(\zeta) - F(\zeta)\Big)\right]\right\}\frac{\Psi}{F(\zeta)} = 0. \tag{S18}$$

An analysis of this equation shows that it can be satisfied if the unknown function $F(\zeta)$ is the generalized Laguerre polynomial $L_n^{|\ell|}(\zeta)$. Such polynomials satisfy the equation

$$\zeta[L_n^\ell(\zeta)]'' + (\ell+1-\zeta)[L_n^\ell(\zeta)]' + nL_n^\ell(\zeta) = 0. \tag{S19}$$

In this case, Eq. (S18) reduces to the form

$$\left\{2k\Phi'_G(z) - \frac{4}{w^2(z)}\big(2n+|\ell|+1\big) + r^2\left(\frac{4}{w^4(z)} - \frac{k^2}{R^2(z)} - k^2\left[\frac{1}{R(z)}\right]'\right)\right.$$
$$\left. +2ik\left[\frac{1}{R(z)} - \frac{w'(z)}{w(z)}\right]\left[|\ell|+1+\frac{2r^2}{w^2(z)}\left(\frac{2[L_n^{|\ell|}(\zeta)]'}{L_n^{|\ell|}(\zeta)} - 1\right)\right]\right\}\Psi' = 0, \tag{S20}$$

where $\Psi'$ is obtained from $\Psi$ by replacing $F(\zeta)$ with $L_n^{|\ell|}(\zeta)$. Explicitly,

$$\Psi' = \frac{C_{n\ell}}{w(z)}\left(\frac{\sqrt{2}r}{w(z)}\right)^{|\ell|} L_n^{|\ell|}\left(\frac{2r^2}{w^2(z)}\right)\exp\left(-\frac{r^2}{w^2(z)}\right)\exp\left(i\left[l\phi + \frac{kr^2}{2R(z)} - \Phi_G(z)\right]\right), \qquad C_{n\ell} = \sqrt{\frac{2n!}{\pi(n+|\ell|)!}}.$$

Wave eigenfunctions with different $n$ or $\ell$ are orthogonal.

Equation (S20) shows that the following differential equations should be satisfied:

$$\frac{1}{R(z)} = \frac{w'(z)}{w(z)}, \qquad \frac{k^2}{R^2(z)} + k^2\left[\frac{1}{R(z)}\right]' = \frac{4}{w^4(z)}, \qquad 2k\Phi'_G(z) = \frac{4}{w^2(z)}\big(2n+|\ell|+1\big). \tag{S21}$$

The initial conditions have the form $w(0) = w_0$, $w'(0) = 0$. The general expressions for the beam parameters are given by (see Refs. [6, 10, 11])

$$w(z) = w_0\sqrt{1+\frac{z^2}{z_R^2}}, \qquad R(z) = z + \frac{z_R^2}{z}, \qquad z_R = \frac{kw_0^2}{2}, \qquad \Phi_G(z) = \big(2n+|\ell|+1\big)\arctan\left(\frac{z}{z_R}\right). \tag{S22}$$

In the general case, the complex radius of curvature of the phase front is also defined by Eq. (S15).

Some formulas in Refs. [5–8] are given with opposite signs.

We should also note the importance of the Hermite-Gauss beams in optics. These beams are solutions of the paraxial wave equation

$$\left(\frac{\partial^2}{\partial x^2} + \frac{\partial^2}{\partial y^2} + 2ik\frac{\partial}{\partial z}\right)\Psi(x,y,z) = 0, \tag{S23}$$

which is equivalent to Eqs. (S1), (S3). One searches the general solution of Eq. (S23) in the form $\Psi(x,y,z) = U_1(x,z)U_2(y,z)$. This solution can be presented in terms of the Hermite polynomials $H_n(\zeta)$ satisfying the following differential equation:

$$H_n''(\zeta) - 2\zeta H_n'(\zeta) + 2nH_n(\zeta) = 0, \qquad n = 0,1,2,\ldots \tag{S24}$$

The wave function satisfying Eq. (S23) is defined by [5, 6]

$$U_1(x,z) = \frac{C_n^{(1)}}{\sqrt{w(z)}}H_n\left(\frac{\sqrt{2}x}{w(z)}\right)\exp\left(-\frac{x^2}{w^2(z)}\right)\exp\left(i\left[\frac{kx^2}{2R(z)} - \Phi_G^{(1)}(z)\right]\right), \qquad C_n^{(1)} = \left(\frac{2}{\pi}\right)^{1/4}\sqrt{\frac{1}{2^n n!}},$$
$$\int U_1^\dagger(x,z)U_1(x,z)dx = 1, \tag{S25}$$

where

$$w(z) = w_0\sqrt{1+\frac{z^2}{z_R^2}}, \qquad R(z) = z + \frac{z_R^2}{z}, \qquad z_R = \frac{kw_0^2}{2}, \qquad \Phi_G^{(1)}(z) = \left(n+\frac{1}{2}\right)\arctan\left(\frac{z}{z_R}\right). \tag{S26}$$

The explicit formula for the total wave function has the form

$$\Psi(x,y,z) = \frac{C_{nm}}{w(z)}H_n\left(\frac{\sqrt{2}x}{w(z)}\right)H_m\left(\frac{\sqrt{2}y}{w(z)}\right)\exp\left(-\frac{x^2+y^2}{w^2(z)}\right)\exp\left(i\left[\frac{k(x^2+y^2)}{2R(z)} - \Phi_G(z)\right]\right), \tag{S27}$$

where the beam parameters are similar to those for Laguerre-Gauss beams:

$$C_{nm} = \sqrt{\frac{2}{2^{n+m}\pi n!m!}}, \qquad \Phi_G(z) = \Phi_G^{(1)}(z) + \Phi_G^{(2)}(z) = (n+m+1)\arctan\left(\frac{z}{z_R}\right). \tag{S28}$$

Wave eigenfunctions with different $n$ or $m$ are orthogonal. The wave eigenfunction of the corresponding fundamental Gaussian note ($n = m = 0$) coincides with that defined by Eqs. (9), (13), and (15).

It is important that expectation values of the OAM operator $l_z = -i\hbar[x\partial/(\partial y) - y\partial/(\partial x)]$ vanish for all Hermite-Gauss beams:

$$< l_z >= -i\hbar\int U_2^\dagger(y,z)U_1^\dagger(x,z)\left(x\frac{\partial}{\partial y} - y\frac{\partial}{\partial x}\right)U_1(x,z)U_2(y,z)dxdy = 0.$$

## II. SOLUTION OF DIFFERENTIAL EQUATIONS

In this Section, we present a detailed derivation of general paraxial wave function for a relativistic electron in a uniform magnetic field. We need to solve the following differential equations:

$$\begin{gathered}\frac{1}{R(z)} = \frac{w'(z)}{w(z)}, \qquad \frac{k^2}{R^2(z)} + k^2\left[\frac{1}{R(z)}\right]' = \frac{4}{w^4(z)} - \frac{4}{w_m^4}, \\ 2k\Phi_G'(z) = \frac{4(\ell+2s_z)}{w_m^2} + \frac{4(2n+|\ell|+1)}{w^2(z)}.\end{gathered} \tag{S29}$$

The substitution of the first equation into the second one leads to the second-order differential equation

$$w''(z) = \frac{4}{k^2}\left[\frac{1}{w^3(z)} - \frac{w(z)}{w_m^4}\right]. \tag{S30}$$

After introducing the new function $v(w(z)) = w'(z)$, taking into account the initial conditions $v(w(0)) = w'(0) = 0$, $w(0) = w_0$, and integrating over $w$, we obtain

$$w''(z) = \frac{dv(w)}{dw}v(w), \qquad [w'(z)]^2 = \frac{4}{k^2}\left[\frac{1}{w_0^2} + \frac{w_0^2}{w_m^4} - \frac{1}{w^2(z)} - \frac{w^2(z)}{w_m^4}\right]. \tag{S31}$$

The equivalent form of this equation reads

$$w'(z) = \pm\frac{2}{kw(z)}\sqrt{-1+\left(\frac{1}{w_0^2}+\frac{w_0^2}{w_m^4}\right)w^2(z) - \frac{w^4(z)}{w_m^4}}. \tag{S32}$$

We can specify the sign with the use of Eq. (S30). Evidently, $w''(0) > 0$ when $w_0 < w_m$ and $w''(0) < 0$ when $w_0 > w_m$. As a result,

$$w(z)w'(z) = \begin{cases} 2C(z)/k & \text{when} \quad w_0 < w_m \\ -2C(z)/k & \text{when} \quad w_0 > w_m \end{cases}, \qquad C(z) = \sqrt{-1+\left(\frac{1}{w_0^2}+\frac{w_0^2}{w_m^4}\right)w^2(z) - \frac{w^4(z)}{w_m^4}} \tag{S33}$$

and

$$X'(z) = \begin{cases} 4C(X(z))/k & \text{when} \quad w_0 < w_m \\ -4C(X(z))/k & \text{when} \quad w_0 > w_m \end{cases}, \qquad C(X(z)) = \sqrt{-1+\left(\frac{1}{w_0^2}+\frac{w_0^2}{w_m^4}\right)X(z) - \frac{X^2(z)}{w_m^4}}, \tag{S34}$$

where $X(z)=w^2(z)$. Let us first consider the case of $w_0<w_m$. With the use of the table of integrals [12], we obtain

$$z=\frac{k}{4}\int_{w_0^2}^{w^2(z)}\frac{dX}{C(X)}=\frac{kw_m^2}{4}\left\{\frac{\pi}{2}-\arcsin\left[\left(\frac{1}{w_0^2}+\frac{w_0^2-2w^2(z)}{w_m^4}\right)\left|\frac{1}{w_0^2}-\frac{w_0^2}{w_m^4}\right|^{-1}\right]\right\}. \quad (S35)$$

This equation results in

$$w(z)=w_0\sqrt{\frac{1}{2}\left[1+\frac{w_m^4}{w_0^4}-\left(\frac{w_m^4}{w_0^4}-1\right)\cos\frac{2z}{z_m}\right]}=w_0\sqrt{\cos^2\frac{z}{z_m}+\frac{w_m^4}{w_0^4}\sin^2\frac{z}{z_m}}, \qquad z_m=\frac{kw_m^2}{2},$$
$$R(z)=kw_m^2\frac{\cos^2\frac{z}{z_m}+\frac{w_m^4}{w_0^4}\sin^2\frac{z}{z_m}}{\left(\frac{w_m^4}{w_0^4}-1\right)\sin\frac{2z}{z_m}}. \quad (S36)$$

A derivation in the case of $w_0>w_m$ is similar. In this case,

$$z=\frac{k}{4}\int_{w_0^2}^{w^2(z)}\frac{dX}{-C(X)}=\frac{kw_m^2}{4}\left\{\frac{\pi}{2}+\arcsin\left[\left(\frac{1}{w_0^2}+\frac{w_0^2-2w^2(z)}{w_m^4}\right)\left|\frac{1}{w_0^2}-\frac{w_0^2}{w_m^4}\right|^{-1}\right]\right\}. \quad (S37)$$

Amazingly, this equation also results in Eq. (S36). Thus, the latter equation remains valid for any relation between $w_0$ and $w_m$.

We can now determine the Gouy phase. Since (see Ref. [12]),

$$\int\frac{dz}{w^2(z)}=\frac{k}{2}\arctan\left(\frac{w_m^2}{w_0^2}\tan\frac{2z}{kw_m^2}\right), \quad (S38)$$

the Gouy phase is defined by

$$\Phi_G(z)=(2n+|\ell|+1)\arctan\left(\frac{w_m^2}{w_0^2}\tan\frac{z}{z_m}\right)+\frac{(\ell+2s_z)z}{z_m}. \quad (S39)$$

In the weak-field limit, $B\rightarrow 0$, $w_m>>w_0$, and $z<<z_m$. Since $\sin z/z_m\approx\tan z/z_m\approx z/z_m$, we obtain

$$w(z)=w_0\sqrt{1+\frac{z^2}{z_R^2}}, \qquad R(z)=z+\frac{z_R^2}{z}, \qquad z_R=\frac{kw_0^2}{2}, \qquad \Phi_G(z)=(2n+|\ell|+1)\arctan\left(\frac{z}{z_R}\right). \quad (S40)$$

We can see that our result, unlike the Landau solution, perfectly reproduces the well-known LG beams in the free space in the weak-field limit.

---


[1] K. Y. Bliokh, I. P. Ivanov, G. Guzzinati, L. Clark, R. Van Boxem, A. Béché, R. Juchtmans, M. A. Alonso, P. Schattschneider, F. Nori, and J. Verbeeck, Theory and applications of free-electron vortex states, Phys. Rep. **690**, 1 (2017).

[2] S. M. Lloyd, M. Babiker, G. Thirunavukkarasu, and J. Yuan, Electron vortices: Beams with orbital angular momentum, Rev. Mod. Phys. **89**, 035004 (2017).

[3] H. Larocque, I. Kaminer, V. Grillo, G. Leuchs, M. J. Padgett, R. W. Boyd, M. Segev, E. Karimi, 'Twisted' electrons, Contemp. Phys. **59**, 126 (2018).

[4] A. J. Silenko, Pengming Zhang, and Liping Zou, Relativistic quantum-mechanical description of twisted paraxial electron and photon beams, Phys. Rev. A **100**, 030101(R) (2019).

[5] A. E. Siegman, *Lasers* (University Science Books, Sausalito, 1986).

[6] H. Kogelnik and T. Li, Laser Beams and Resonators, Appl. Opt. **5**, 1550 (1966).

[7] J. Alda, Laser and Gaussian Beam Propagation and Transformation, in *Encyclopedia of Optical Engineering*, vol. 2, ed. by R. G. Driggers, C. Hoffman, and R. Driggers (Marcel Dekker Inc., New York, 2003), pp. 999-1013.

[8] F. Pampaloni, J. Enderlein, Gaussian, Hermite-Gaussian, and Laguerre-Gaussian beams: A primer, arXiv:physics/0410021 (2004).

[9] L. D. Landau, E. M. Lifshitz, *Quantum Mechanics. Non-Relativistic Theory*, 3rd ed. (Pergamon Press, Oxford, 1977), pp. 458-461.

[10] L. Allen, M. W. Beijersbergen, R. J. C. Spreeuw, J. P. Woerdman, Orbital angular momentum of light and the transformation of Laguerre-Gaussian laser modes, Phys. Rev. A **45**, 8185 (1992).

[11] S. M. Barnett, M. Babiker and M. J. Padgett, Optical orbital angular momentum, Phil. Trans. R. Soc. A **375**, 20150444 (2017).

[12] I. S. Gradshteyn and I. M. Ryzhik, *Table of Integrals, Series, and Products*, 8th ed. (Academic Press, Amsterdam, 2015).
